# Supplementary material for: Transformers as Graph-to-Graph Models
Source: arXiv:2310.17936 source file (2023-10-27)
Supplement: Supplementary file 1 [file supplementary.tex]

\setcounter{section}{0}
\onecolumn
\begin{appendices}

\end{appendices}
